# Supplementary material for: FastFold: Reducing AlphaFold Training Time from 11 Days to 67 Hours
Source: arXiv:2203.00854 source file (2023-02-05)
Supplement: Supplementary file 1 [file appendix.tex]

\appendices

\section{Algorithm Details of Evoformer}
\label{evoformer_algo}

\rebuttal{We present algorithm details of Outer Product Mean and Triangular Update in evoformer, where we use the following conventions. Indices $i$, $j$ operate on the residue dimension, indices $s$ on the sequence dimension. We use \{$\boldsymbol{m}_{si}$\} to denote all pair representations and \{$\boldsymbol{z}_{si}$\} to denote all MSA representations. And we use $\otimes$ for the outer product and $\odot$ for the element-wise multiplication.}

\rebuttal{Algorithm \ref{algo_msa_row} shows row-wise gated self-attention. The calculation process for the column-wise attention and the attention in the Template Stack is similar, with some differences in the attention bias.}

\begin{algorithm}
 \caption{\rebuttal{Algorithm for MSA Row Attention}}
 \begin{algorithmic}[1]
 \label{algo_msa_row}

 \REQUIRE \{$\boldsymbol{m}_{si}$\}, \{$\boldsymbol{z}_{ij}$\}, $N_{head}$
 \ENSURE  \{$\boldsymbol{m}_{si}$\}
  \STATE $\boldsymbol{q}_{si}^{h}$, $\boldsymbol{k}_{si}^{h}$, $\boldsymbol{v}_{si}^{h}$ = Linear(LayerNorm($\boldsymbol{m}_{si}$)),   $h \in \{1..N_{head}\}$
  \STATE $b_{ij}^{h}$ = Linear(LayerNorm($\boldsymbol{z}_{ij}$))   \textit{\# Attention Bias}
  \STATE $\boldsymbol{g}_{si}^{h}$ = sigmoid(Linear($\boldsymbol{m}_{si}$))
  \STATE $a_{sij}^{h}$ = softmax${}_{j}(({\boldsymbol{q}_{si}^{h}}^{T} \boldsymbol{k}_{sj}^{h} + b_{ij}^{h})/\sqrt{c})$
  \STATE $\boldsymbol{o}_{si}^{h}$ = $\boldsymbol{g}_{si}^{h} \odot \sum_{j} a_{sij}^{h} \boldsymbol{v}_{sj}^{h}$
  \STATE $\boldsymbol{m}_{si}$ = Linear(concat${}_{h}$($\boldsymbol{o}_{si}^{h}$))
 \RETURN $\boldsymbol{m}_{si}$
 \end{algorithmic} 
\end{algorithm}

The algorithm details of Outer Product Mean and Triangular Update Module are shown in Algorithm \ref{algo_outer_product_mean} and \ref{algo_triangular}.

\begin{algorithm}
 \caption{Algorithm for Outer Product Mean}
 \begin{algorithmic}[1]
 \label{algo_outer_product_mean}

 \REQUIRE \{$\boldsymbol{m}_{si}$\}
 \ENSURE  \{$\boldsymbol{z}_{ij}$\}
  \STATE $\boldsymbol{m}_{si}$ = LayerNorm($\boldsymbol{m}_{si}$)
  \STATE $\boldsymbol{a}_{si}$, $\boldsymbol{b}_{si}$ = Linear($\boldsymbol{m}_{si}$)
  \STATE $\boldsymbol{o}_{ij}$ = mean${}_{s}$($\boldsymbol{a}_{si} \otimes \boldsymbol{b}_{sj}$)
  \STATE $\boldsymbol{z}_{ij}$ = Linear(flatten($\boldsymbol{o}_{ij}$))
 \RETURN $\boldsymbol{z}_{ij}$
 \end{algorithmic} 
\end{algorithm}
 
\begin{algorithm}
 \caption{\rebuttal{Algorithm for Triangular Update Module}}
 \begin{algorithmic}[1]
 \label{algo_triangular}

 \REQUIRE \{$\boldsymbol{z}_{ij}$\}
 \ENSURE  \{$\boldsymbol{z}_{ij}$\}
  \STATE $\boldsymbol{z}_{ij}$ = LayerNorm($\boldsymbol{z}_{ij}$)
  \STATE $\boldsymbol{g}_{ij}$ = sigmoid(Linear($\boldsymbol{z}_{ij}$))
  \STATE $\boldsymbol{a}_{ij}$, $\boldsymbol{b}_{ij}$ = sigmoid(Linear($\boldsymbol{z}_{ij}$)) $\odot$ Linear($\boldsymbol{z}_{ij}$)
  \STATE $\boldsymbol{z}_{ij}$ = $\boldsymbol{g}_{ij}$ $\odot$ Linear(LayerNorm($\sum_{k}\boldsymbol{a}_{ik} \odot \boldsymbol{b}_{jk}$))
 \RETURN $\boldsymbol{z}_{ij}$
 \end{algorithmic} 
 \end{algorithm}
